# Supplementary material for: Scalable Time-Lock Puzzle
Source: arXiv:2308.01280 source file (2025-05-23)
Supplement: Supplementary file 1 [file evaluation--full.tex]

\section{Full Analysis of Asymptotic Costs}\label{sec:Full-Analysis-of-Asymptotic-Costs}

\subsection{Computation Cost.}
Below, we analyze the computation complexity of the following four schemes: 
\begin{enumerate*}[label=(\arabic*)]
\item the original TLP of \citeauthor{Rivest:1996:TPT:888615}~\cite{Rivest:1996:TPT:888615}, 
\item the C-TLP of \citeauthor{Abadi-C-TLP}~\cite{Abadi-C-TLP}, 
\item our \gc presented in Section~\ref{subsec:gc-tlp-protocol} on page~\pageref{subsec:gc-tlp-protocol}, and 
\item our ED-TLP presented in Section~\ref{subsec:efficient-delegated-time-locked-puzzle} on page~\pageref{subsec:efficient-delegated-time-locked-puzzle}.
\end{enumerate*}

\begin{itemize}[leftmargin=5mm]
\item \textit{\brokenuline{RSA-based Time-Lock Puzzle (TLP)}}.
Client \cl in the set\-up phase performs modular exponentiation (over $\mathbb{Z}_{\phi(N)}$) for each puzzle.
Thus, for $z$ puzzles it performs $O(z)$ modular exponentiation in this phase.
\cl in the puzzle generation phase, for each puzzle, invokes an instance of symmetric-key encryption, performs a single modular exponentiation, and a modular addition.
Thus, for $z$ puzzles, \cl invokes each of the above three operations (i.e., symmetric-key encryption, exponentiation, and addition) $O(z)$ times.
Server \se in the puzzle-solving phase, to solve $i$-th puzzle (a) performs $T_i = S\cdot \Delta_i$ number of squaring modulo $N$, (b) performs a single modular subtraction, and (c) single symmetric-key decryption.
Thus, for $z$ puzzles, \se performs $O(S\cdot\sum_{i=1}^z\Delta_i)$ modular squaring/exponentiation, and $O(z)$ modular subtraction and symmetric-key decryption.

\item \textit{\brokenuline{Chained Time-Lock Puzzle (\ctlp)}}.
\cl in the setup, performs single exponentiation (over $\mathbb{Z}_{\phi(N)}$) to generate parameters for $z$ puzzles.
In the puzzle generation phase, \cl invokes $O(z)$ instances of symmetric-key encryption, performs $O(z)$ modular exponentiation over $\mathbb{Z}_N$ and carries out $O(z)$ modular addition.
In the same phase, \cl invokes $O(z)$ instances of the hash function.
Thus, the total computation complexity of \cl in the puzzle generation phase is $O(z)$.
For \se to solve $z$ puzzles, it performs $O(z\cdot S\cdot \Delta)$ modular squaring over $\mathbb{Z}_N$, carries out $O(z)$ modular addition, and invokes $O(z)$ instances of symmetric-key decryption.
Therefore, the total computation complexity of \se is $O(z\cdot S\cdot \Delta)$.
The verification cost  mainly involves invoking $O(z)$ instances of the hash function.

\item \brokenuline{\textit{Our \gc}}.
\cl in the setup phase (Phase~\ref{GC-TLP::step::setup}), performs $z$ exponentiation (over $\mathbb{Z}_{\phi(N)}$) to generate the parameters (i.e., $\ex_1$, $\ldots$, $\ex_z$) for $z$ puzzles.
In the generate puzzle phase (Phase~\ref{GC-TLP::step::Generate-Puzzle}), \cl invokes $O(z)$ instances of symmetric-key encryption, performs $O(z)$ modular exponentiation over $\mathbb{Z}_N$ and conducts $O(z)$ modular addition.
In this phase, \cl invokes  $O(z)$ instances of the hash function.
So, its total computation complexity in the puzzle generation phase is $O(z)$.
For \se to solve $z$ puzzles (in Phase~\ref{GC-TLP::step::Solve-Puzzle}), it performs $O(S\cdot \sum_{i=1}^z\bar{\Delta}_i)$ modular squaring over $\mathbb{Z}_N$, carries out $O(z)$ modular addition, and invokes $O(z)$ instances of symmetric-key decryption, where $\bar{\Delta}_i<{\Delta}_i$ when $i > 1$.
Hence, \se's total computation complexity is $O(S\cdot\sum_{i=1}^z\bar{\Delta}_i)$.
The prove phase (Phase~\ref{GC-TLP::step::prove-}) imposes a negligible cost to \se.
The verify phase (Phase~\ref{GC-TLP::step::verify-}) cost involves invoking $O(z)$ instances of the hash function.

\item \brokenuline{\textit{Our \dgc}}.
\cl's cost in the setup phase (Phase~\ref{DGC-TLP::step::Client-side-Setup}) is negligible, as it involves generating a single secret key.
\cl in the client-side delegation phase (Phase~\ref{DGC-TLP::step::Client-side-Delegation}) invokes $O(z)$ instances of symmetric-key encryption.
\tpc in the helper-side setup phase (Phase~\ref{DGC-TLP::step::Helper-side-Setup}), performs $z$ exponentiation (over $\mathbb{Z}_{\phi(N)}$) to generate the parameters for $z$ puzzles. \tpc in the helper-side puzzle generation phase (Phase~\ref{DGC-TLP::Generate-Puzzle-}), invokes $O(z)$ instances of symmetric-key encryption, performs $O(z)$ modular exponentiation over $\mathbb{Z}_N$ and carries out $O(z)$ modular addition.
In this phase, \tpc also invokes $O(z)$ instances of the hash function.
\se's computation cost in the delegation phase (Phase~\ref{DGC-TLP::step::Server-side-Delegation})  mainly involves $O(z)$ additions.
Its cost in the retrieve phase (Phase~\ref{DGC-TLP::step::retrive}) mainly involves $O(z)$ invocations of the decryption algorithm of symmetric key encryption.
 
The cost of \tps in the solve puzzle phase (Phase~\ref{DGC-TLP::step::Solve-Puzzle}) includes $O\left(S\cdot\sum_{i=1}^z\bar{\Delta}_i\right)$ modular exponentiation, $O(z)$ modular addition, and $O(z)$ symmetric key decryption.
Its cost in the prove and register phases (Phases~\ref{prove-D} and~\ref{DGC-TLP::step::Register-Puzzle}) is negligible.
The cost of \scc in the verify phase (Phase~\ref{verify-D})
involves $O(z)$ addition and $O(z)$ invocations of the hash function.
Its cost in the pay phase (Phase~\ref{DGC-TLP::step::pay}) is negligible.
\end{itemize}

Hence, \begin{enumerate*}[label=(\arabic*)]
    \item \dgc has the lowest client-side setup cost, 
    \item \dgc has the lowest server-side cost,
    \item TLP, \ctlp, our \gc, and \dgc have the same computation complexity in the puzzle-solving phase (but the last three schemes impose much lower costs than TLP, in the multi-client setting), and
    \item \ctlp, our \gc, and \dgc have the same verification cost. 
\end{enumerate*}

\subsection{Communication Cost.} 

\begin{itemize}
\item \textit{\brokenuline{RSA-based Time-Lock Puzzle (TLP)}}.
The total communication cost of the TLP is $O(z)$, as \cl for each puzzle sends to \se two values, 
\begin{enumerate*}[label=(\arabic*)]
    \item an element of $\mathbb{Z}_N$ (whose size is about $2048$ bits) and
    \item ciphertext of symmetric-key encryption (whose size is about $256$ bits).
\end{enumerate*}

\item \brokenuline{\textit{C-TLP and our \gc}}.
In the C-TLP and \gc, for each puzzle, \cl sends to \se a commitment (whose size is about $256$ bits), an element of $\mathbb{Z}_N$ and ciphertext of symmetric-key encryption.
In the proving phase, \se sends an opening of a commitment (with the total size of $256+|m|$, where $|m|$ is the plaintext solution's size).
Thus, the total communication cost for $z$ puzzles in the C-TLP and \gc is $O(z)$.

\item \brokenuline{\textit{Our \dgc}}.
In the \dgc, \cl in the client-side delegation phase (Phase~\ref{DGC-TLP::step::Client-side-Delegation}) for each puzzle sends a ciphertext of symmetric-key encryption to \tpc.
\se in the server-side delegation phase (Phase~\ref{DGC-TLP::step::Server-side-Delegation}) deploys to the blockchain a smart contract \scc.
It also sends to \scc:
\begin{enumerate*}[label=(\arabic*)]
    \item $z$ values $T_1$, $\ldots$, $T_z$, where each value is a few bits long, and
    \item a single address $\adr_\scc$ to \tps.
\end{enumerate*}
\tpc in the helper-side puzzle generation phase (Phase~\ref{DGC-TLP::Generate-Puzzle-}) sends to \tps a vector \puzzvec of $z$ puzzles, where each puzzle is a pair containing an element of $\mathbb{Z}_N$ and a ciphertext of symmetric-key encryption.
In the same phase, it sends to \scc a vector \commvec of $z$ commitments. \tps in the register puzzle phase (Phase~\ref{DGC-TLP::step::Register-Puzzle}) sends to \scc a vector of pairs where each pair contains a ciphertext of symmetric-key encryption and a random value (of size $256$-bit).
Thus, \dgc's total communication cost in the $z$-puzzle setting is $O(z)$.
\end{itemize}
Hence, in the $z$-puzzle setting, all four schemes' overall communication complexity is $O(z)$, while \dgc has the lowest
\begin{enumerate*}[label=(\arabic*)]
\item client-side and 
\item server-side communication costs,
\end{enumerate*}
because in this scheme \cl and \se send messages of much shorter length than they do in the other three schemes.
