# Supplementary material for: Scalable Time-Lock Puzzle
Source: arXiv:2308.01280 source file (2025-05-23)
Supplement: Supplementary file 2 [file CEDG-instantiation.tex]

\section{Instantiation of \ced}\label{sec::instantiation-of-ced}
A good candidate is to consider how the helper compares to the (most capable) server that determines $S$ when creating the puzzle.
Assuming $aux_{ID}$ contains $S_{ID}$, the number of squarings per second helper $\tps_{\st ID}$ is capable of, we set $\ced(ToC, S, \Delta, aux_{\st ID})\rightarrow \Delta \cdot \left( 1+\frac{S_{ID}}{S}\right)$.
This instantiation can also include a fixed delay to indicate how long until a busy helper will be available, specified as part of $aux_{ID}$.
